# Supplementary material for: A Survey of Quantum Theory Inspired Approaches to Information Retrieval
Source: arXiv:2007.04357 source file (2020-07-08)
Supplement: Supplementary file 1 [file Appendix.tex]

\section{Appendix}
Consider a state vector in two different basis of a two dimensional Hilbert space, $$ \ket{\psi} = a\ket{A}+b\ket{B} = c\ket{C}+d\ket{D}$$ We want to represent the vectors of one basis in terms of the other. To do that, consider the vector orthogonal to $\ket{\psi}$, which is $\ket{\widetilde{\psi}} = b\ket{A}-a\ket{B} = d\ket{C}-c\ket{D}$. Using these two expressions, we get 
\begin{align}\label{c,d}
\ket {C} &= c\ket{\psi} + d\ket{\widetilde{\psi}} \\ \nonumber 
\ket {D} &= d\ket{\psi} - c\ket{\widetilde{\psi}}
\end{align}
Substituting $\ket{\psi} = a\ket{A}+b\ket{B}$ and $\ket{\widetilde{\psi}} = b\ket{A}-a\ket{B}$ in \ref{c,d}, we get
\begin{align}
\ket {C} &= (ac+bd)\ket{A} + (bc-ad)\ket{B} \\ \nonumber
\ket {D} &= (ad-bc)\ket{A} + (ac+bd)\ket{B}
\end{align}

We can thus represent one basis of a Hilbert Space in terms of another basis.
